# Supplementary material for: Decision Procedures for Path Feasibility of String-Manipulating Programs with Complex Operations
Source: arXiv:1811.03167 source file (2018-11-07)
Supplement: Supplementary file 1 [file replace2pt-appendix.tex]

%!TEX root = POPL19.tex

%\section{Proof of Proposition~\ref{prop-replace-pt}: From $\replaceall_p$ to \PT}

\subsection*{Proof for expressing $\replaceall_p$ by \PT} \label{appendix:replace2pt}

Let $p$ be a fixed patten and $\replaceall_p(sub, rep)$ be an instance of the $\replaceall$ function, where $sub, rep$ are the subject and replacement respectively. W.l.o.g. we assume that $p$ is given by an \FA{} $\Aut_0$. For simplicity, we assume that $\varepsilon$ does not belong to $\Lang(\Aut_0)$. Our goal is to construct a \PT{} $\Transducer_p = (\controls, q_0, \finals, \transrel)$ to simulate $\replaceall_p(sub, rep)$.

Intuitively, $\Transducer_p$ takes $sub$ as the input string and $rep$ as a parameter. If $sub \in \Sigma^* \backslash (\Sigma^\ast e_0 \Sigma^\ast)$, then $\Transducer_p$ outputs $sub$. Otherwise, $\Transducer_p$ parses $sub$ into the substrings $v_1 u_1 v_2 u_2 \ldots v_l u_l v_{l+1}$ such that
\begin{itemize}
	\item for each $j \in [l]$, $u_j$ is the leftmost and longest matching of $p$ in the string $(v_1 u_1 \ldots v_{j-1} u_{j-1})^{-1} v$,
	\item $v_{l+1} \in \Sigma^* \backslash (\Sigma^\ast e_0 \Sigma^\ast)$,
\end{itemize}
and outputs $v_1\cdot rep \cdot v_2 \cdot rep \ldots v_l \cdot rep \cdot v_{l+1}$. 

$\Transducer_p$ is essentially the extension of the parsing automaton $\Aut_p$ constructed in \cite{CCHLW18} with outputs.

Since the construction is very similar to that of $\Aut_p$ in \cite{CCHLW18}, we will only give an intuitive description of the behaviour of $\Transducer_p$ below and encourage the readers to check $\Aut_p$ in \cite{CCHLW18} for details.
%We start with an automaton that can have an infinite number of states and describe the automaton as starting new ``threads'', i.e., run multiple copies of $\Aut_0$ on the input word (similar to alternating automata).
%We also show how this automaton can be implemented using only a finite number of states.
Intuitively, in order to search for the leftmost and longest matching of $p$ (i.e. $\Aut_0$), $\Transducer_{p}$ behaves as follows.
\begin{itemize}
\item $\Transducer_{p}$ has two modes, ``$\searchleft$'' and ``$\searchlong$'', which intuitively means searching  for the first and last position of the leftmost and longest matching of $e_0$ respectively.
\item When in the ``$\searchleft$'' mode, $\Transducer_{p}$ starts a new thread of $\Aut_0$ in each position and records \emph{the set of states} of the threads into a vector.
    In addition, it nondeterministically makes a ``leftmost'' guessing, that is, guesses that the current position is the first position of the leftmost and longest matching. Before making such a guessing, $\Transducer_{p}$ outputs each letter it reads.
    If it makes such a guessing, it enters the ``$\searchlong$'' mode, runs the thread started in the current position and searches for the last position of the leftmost and longest matching.
    Moreover, it stores in a set $S$ the union of the sets of states of all the threads that were started before the current position and continues running these threads to make sure that, in these threads, the final states will not be reached (thus, the current position is indeed the first position of the leftmost and longest matching).
\item When in the ``$\searchlong$'' mode, $\Transducer_p$ runs a thread of $\Aut_{0}$ to search for the last position of the leftmost and longest matching.
    If the set of states of the thread contains a final state, then $\Transducer_p$ nondeterministically guesses that the current position is the last position of the leftmost and longest matching.
    If it makes such a guessing, then it resets the set of states of the thread and starts a new round of searching for the leftmost and longest matching.
    In addition, it stores the original set of states of the thread into a set $S$ and continues running the thread to make sure that in this thread, the final states  will not be reached (thus, the current position is indeed the last position of the leftmost and longest matching). Before making such a guessing in the ``$\searchlong$'' mode, $\Transducer_p$ always outputs $\epsilon$. On the other hand, when the guessing is made, $\Transducer_p$ outputs the parameter $rep$. 
	%
%	\item when a thread $i$ enters a final state, a matching of $e$ is found, $\cB_e$ nondeterministically guesses whether this matching is the leftmost matching or the longest matching,
	%
%	\item if $\cB_e$ makes a ``leftmost and longest'' guessing, then $\cB_e$ forgets all the other threads that were started later than the thread $i$, and continues running the thread $i$ and all the threads that were started earlier than the thread $i$ to make sure that final states will not be reached and the ``leftmost and longest'' guessing is correct,
%
%	\item if $\cB_e$ makes a ``leftmost and non-longest'' guessing, then $\cB_e$ forgets all the other threads that were started later than the thread $i$, and continues running all the threads that were started earlier than the thread $i$ to make sure that final states will not be reached and the ``leftmost'' guessing is correct, in addition, it continues running the thread $i$ and searching for the longest matching,
%
%	\item if $\cB_e$ makes a ``non-leftmost'' guessing, then $\cB_e$ forgets the thread $i$ and all the other threads that were started later than the thread $i$, and continues running all the threads that were started earlier than the thread $i$ and searching for the leftmost matching,
	%
	\item Since the length of the vectors of the sets of states of the threads may become unbounded, in order to obtain a finite state automaton, the following trick is applied.
    Suppose that the vector is $S_1 S_2 \cdots S_n$.
    For each pair of indices $i, j: i < j$ and each $q \in S_i \cap S_j$, remove $q$ from $S_j$.
    The application of this trick is justified by the following arguments: Since $q$ occurs in both $S_i$ and $S_j$ and the thread $i$ was started before the thread $j$, even if from $q$  a final state can be reached in the future, the position where the thread $j$ was started \emph{cannot} be the first position of the leftmost and longest matching, since the state $q$ is also a state of the thread $i$ and the position where the thread $i$ was started is before the position where the thread $i$ was started.
\end{itemize}

Since the size of $\Transducer_p$ is the same as the parsing automaton $\Aut_p$ in \cite{CCHLW18}, and it was shown in  \cite{CCHLW18} that the size of $\Aut_p$ is $2^{\bigO(|p|^c)}$ for some constant $c > 0$, we conclude that the size of $\Transducer_p$ is $2^{\bigO(|p|^c)}$.
