# Supplementary material for: Decision Procedures for Path Feasibility of String-Manipulating Programs with Complex Operations
Source: arXiv:1811.03167 source file (2018-11-07)
Supplement: Supplementary file 2 [file sec-2way-appendix.tex]

%!TEX root = main.tex

\section{Details in Section~\ref{sec-2way}} \label{appendix:sec-2way}

\paragraph{Claim.} For each tuple of strings $(w, w_1,\cdots, w_\arity)$, $(w, w_1,\cdots, w_\arity) \in \Pre_\Transducer(\Aut)$ iff there are $\conacc_{x_1}, \cdots, \conacc_{x_\arity} \subseteq Q' \times Q'$ and $q \in F$ such that $w \in \Lang(\cB_{\Transducer, \conacc_{x_1}, \cdots, \conacc_{x_\arity}, q})$ and $w_i \in \Lang(\Aut[\conacc_{x_i}])$ for each $i \in [\arity]$, where $\Aut[\conacc_{x_i}]=((Q', \delta'), \conacc_{x_i})$.

\begin{proof}
Recall $\Transducer = (X, Q, q_0, F, \delta)$ with $X= \{x_1,\cdots, x_\arity\}$ and $\Aut =( (Q', \delta'), \conacc)$. 
Suppose $\Gamma = \Sigma \cup X$. 

Let $w, w_1, \cdots, w_\arity$ be strings and $w = a_1 \cdots a_n$ with $a_i \in \Sigma$ for each $i \in [n]$.

\smallskip

\noindent {\it ``Only if'' direction}: 

\smallskip

Assume that $(w, w_1,\cdots, w_r) \in \Pre_\Transducer(\Aut)$.

From the definition of $\Pre_\Transducer(\Aut)$, since $T$ is functional, we know that there are a unique string $w'$, and an accepting run of $\Transducer$ on $w$, equipped with the parameters $w_1,\cdots, w_r$, say $(q_0, i_0, w'_0),\ldots, (q_m, i_m, w'_m) \in \controls \times [n+1] \times \Gamma^*$, such that 
\begin{itemize}
\item $i_0=0$, $i_m = n+1$, $q_m \in F$, 
\item let $a_0 = \EndLeft$ and $a_{n+1} = \EndRight$,  then $w'_0 = w'_m = \varepsilon$, and for every $j \in [0, m-1]$, $(q_j, a_{i_j}, dir_{i_j}, q_{j+1}, w'_j) \in
        \transrel$ and $i_{j+1} = i_j + dir_{i_j}$ for some $dir_{i_j} \in \{\Left, \Stay, \Right\}$, 
 \item $w'$ is the output corresponding to the run, that is, $ w' = w''_1 \cdots w''_{m-1}$, where for each $j \in [m-1]$, $w''_j = w'_j[w_1/x_1,\ldots, w_r/x_r]$,
 \item  $w' \in \Lang(\Aut)$.
\end{itemize}

For each $j \in [m-1]$, suppose $w'_j = w'_{j, 1} x_{i_{j, 1}} \ldots x_{i_{j, s_j}} w'_{j, s_j+1}$ such that $w'_{j,1}, \ldots, w'_{j, s_j +1 } \in \ialphabet^*$.

Since $ w' = w''_1 \cdots w''_{m-1}$ and $w''_j = w'_j[w_1/x_1,\ldots, w_r/x_r]$, 
from $w' \in \Lang(\Aut)$, we deduce that for each $\omega = (p, p') \in \conacc$, there is a state sequence 
{\small
$$q'_{\omega, 1, 0}, \ldots, q'_{\omega, 1, 2s_1+1}, q'_{\omega, 2, 1}, \ldots, q'_{\omega, 2, 2s_2+1}, \ldots, q'_{\omega, m-1, 1}, \ldots, q'_{\omega, m-1, 2s_{m-1}+1} \in Q'$$ 
}
\begin{itemize}
\item $q'_{\omega,1, 0}= p$, 
\item for each $j \in [m-1]$ and $j' \in [s_j]$, 
$$q'_{\omega, j, 2(j'-1)} \xrightarrow[\Aut]{w'_{j, j'}} q'_{\omega, j, 2j'-1} \xrightarrow[\Aut]{w_{i_{j, j'}}} q'_{\omega, j, 2j'},$$ 
and $q'_{\omega, j, 2s_j} \xrightarrow[\Aut]{w'_{j, s_j+1}} q'_{\omega, j, 2s_j+1}$,  where $q'_{\omega, j, 0} = q'_{\omega, j-1, 2s_{j-1}+1}$ if $j > 1$, 
%and $q'_{\omega, j, 2j'-1} \xrightarrow[\Aut]{\conacc_{i_{j, j'}}} q'_{\omega, j, 2j'}$ means $(q'_{\omega, j, 2j'-1}, q'_{\omega, j, 2j'}) \in \conacc_{i_{j, j'}}$,
%
\item $q'_{\omega, m-1, 2s_{m-1}+1} = p'$.
\end{itemize}
For each $i' \in [r]$, let $\conacc_{x_{i'}}$ be the set of state pairs $(q'_{\omega, j, 2j'-1}, q'_{\omega, j, 2j'})$ such that $\omega \in \conacc$, $j \in [m-1]$, and $x_{i_{j, j'}} = x_{i'}$. Evidently, for each $i' \in [r]$, $w_{i'}$ is accepted by $\Aut[\conacc_{x_{i'}}]$.
With $\conacc_{x_1}, \ldots, \conacc_{x_r}$, we can construct the conjunctive \SSA{} $\cB_{\Transducer, \Aut, \conacc_{x_1}, \ldots, \conacc_{x_r}, q_m} = ((\controls'', \transrel''), \conacc'')$ as in Section~\ref{sec-2way}, where $\conacc'' = \{((q_0, p), (q_m, p') ) \mid (p, p') \in \conacc\}$. From the construction of $\cB_{\Transducer, \Aut, \conacc_{x_1}, \ldots, \conacc_{x_r}, q_m}$, we know that $\cB_{\Transducer, \Aut, \conacc_{x_1}, \ldots, \conacc_{x_r}, q_m}$ contains the following transitions: 
\begin{itemize}
\item $((q_0, q'_{\omega, j, 0}), a_{i_0}, dir_{i_0}, (q_1, q'_{\omega, j, 0}))$,
\item $((q_j, q'_{\omega, j, 0}), a_{i_j}, dir_{i_j}, (q_{j+1}, q'_{\omega, j, 2s_{j}+1}))$ for each $j \in [m-1]$ and $\omega \in \conacc$.
%\item $(q_{m-1},q'), a_{i_m}, )$
\end{itemize}
Therefore, for each $\omega = (p, p') \in \conacc$, 
$$((q_0, q'_{\omega, 1, 0}), i_0), \ldots, ((q_m, q'_{\omega, m-1, 2s_{m-1}+1}), i_m)$$ 
is an accepting run of $((\controls'', \transrel''), \{((q_0, p), (q_m, p'))\})$ on $w$. 
We then conclude that $w$ is accepted by $\cB_{\Transducer, \Aut, \conacc_{x_1}, \ldots, \conacc_{x_r}, q_m}$.

\smallskip

\noindent {\it ``If'' direction}: 

\smallskip

Suppose that there are $\conacc_{x_1},\cdots, \conacc_{x_r} \subseteq Q' \times Q'$ and $q \in F$ such that $w \in \Lang(\cB_{\Transducer, \conacc_{x_1}, \cdots, \conacc_{x_r}, q})$ and $w_i \in \Lang(\Aut[\conacc_{x_i}])$ for each $i \in [r]$. 

Since $\Lang(\cB_{\Transducer, \conacc_{x_1}, \cdots, \conacc_{x_r}, q})=\Lang(\Aut'')$, we know that  there are an accepting run of $\Transducer$ on $w$, 
say $(q_0, i_0, w'_0),\ldots, (q_m, i_m, w'_m) \in \controls \times [n+1] \times \Gamma^*$, such that 
\begin{itemize}
\item $i_0=0$, $i_m = n+1$, $q_m \in F$, $w'_0 = \epsilon$,
\item let $a_0 = \EndLeft$ and $a_{n+1} = \EndRight$,  then for every $j \in [m-1]$, $(q_j, a_{i_j}, dir_{i_j}, q_{j+1}, w'_j) \in
        \transrel$ and $i_{j+1} = i_j + dir_{i_j}$ for some $dir_{i_j} \in \{\Left, \Stay, \Right\}$, 
 \item  let $\omega =(p, p') \in \conacc$,  and for each $j \in [m-1]$, $w'_j = w'_{j, 1} x_{i_{j, 1}} \ldots w'_{j, s_j} x_{i_{j, s_j}} w'_{j, s_j + 1}$ such that $w'_{j, j'} \in \ialphabet^*$ for each $j' \in [s_j+1]$, then there are states 
 $$q'_{\omega, 1, 0}, q'_{\omega, 1,1}, \ldots, q'_{\omega, 1, 2s_1 +1}, \ldots,  q'_{\omega, m-1, 1},  \ldots, q'_{\omega, m-1, 2s_{m-1} +1} \in \controls'$$
 satisfying that 
 \begin{itemize}
\item $q'_{\omega, 1, 0} = p$, $q'_{\omega, m-1, 2s_{m-1} +1} = p'$, and 
\item for each $j \in [m-1]$, 
{\small
$$q'_{\omega, j, 0} \xrightarrow[\Aut]{w'_{j, 1} } q'_{\omega, j, 1} \xrightarrow{\conacc_{x_{i_{j, 1}}}} q'_{\omega, j, 2}\ \ldots\ q'_{\omega, j, 2s_j-1} \xrightarrow{\conacc_{x_{i_{j, s_j}}}} q'_{\omega, j, 2s_j} \xrightarrow[\Aut]{w'_{j, s_j + 1}} q'_{\omega, j, 2s_j+1},$$ 
}
\end{itemize}
where $q'_{\omega, j, 0} = q'_{\omega, j-1, 2s_{j-1}+1}$ if $j > 1$, and $q'_{\omega, j, 2j'-1} \xrightarrow{\conacc_{x_{i_{j, j'}}}} q'_{\omega, j, 2j'}$ means $(q'_{\omega, j, 2j'-1} , q'_{\omega, j, 2j'}) \in \conacc_{x_{i_{j, j'}}}$ for each $j' \in [s_j]$.
\end{itemize}

Let $w'$ be the output of the run on $w$, equipped with the parameters $w_1,\ldots, w_r$, more precisely, $w' = w''_1 \cdots w''_{m-1}$ such that  $w''_j = w'_j[w_1/x_1, \ldots, w_r/x_r]$ for each $j \in  [m-1]$. From the fact that $w_i \in \Lang(\Aut[\conacc_{x_i}])$ for each $i \in [r]$, we deduce that for each $\omega = (p,p') \in \conacc$ and $j \in [m-1]$, $q'_{\omega, j, 0} \xrightarrow[\Aut]{w''_j} q'_{\omega, j, 2s_j+1}$.
Therefore, for each $\omega = (p,p') \in \conacc$, $p \xrightarrow[\Aut]{w'} p'$. From this, we deduce that $w'$ is accepted by $\Aut=((Q', \delta'), \conacc)$.
Consequently, $(w, w_1,\cdots, w_r) \in \Pre_\Transducer(\Aut)$.
\end{proof}
